# Supplementary material for: Magneto-optics of a Weyl semimetal beyond the conical band approximation: the case study of TaP
Source: arXiv:1912.07327 source file (2020-04-10)
Supplement: Supplementary file 1 [file SM.pdf]

# Magneto-optics of a Weyl semimetal beyond the conical band approximation: the case study of TaP

## Supplementary Material

S. Polatkan,[1] M. O. Goerbig,[2] J. Wyzula,[3] R. Kemmler,[1] L. Z. Maulana,[1] B. A. Piot,[3] I. Crassee,[3] A. Akrap,[4] C. Shekhar,[5] C. Felser,[5] M. Dressel,[1] A. V. Pronin,[1] and M. Orlita[3,6]

[1] *1. Physikalisches Institut, Universität Stuttgart, Pfaffenwaldring 57, 70569 Stuttgart, Germany*
[2] *Laboratoire de Physique des Solides, Université Paris-Saclay, CNRS UMR 8502, 91405 Orsay Cedex, France*
[3] *Laboratoire National des Champs Magnétiques Intenses, CNRS-UGA-UPS-INSA-EMFL, 25 rue des Martyrs, 38042 Grenoble, France*
[4] *Department of Physics, University of Fribourg, Chemin du Musée 3, CH-1700 Fribourg, Switzerland*
[5] *Max Planck Institut für Chemische Physik Fester Stoffe, 01187 Dresden, Germany*
[6] *Charles University, Faculty of Mathematics and Physics, Institute of Physics, Ke Karlovu 5, 121 16 Prague 2, Czech Republic*

In the Supplementary Materials provided here we discuss the details of the theoretical calculations, band structure parameters of TaP and the results of magneto-transport experiments.

## I. DETAILS OF THE LOW-ENERGY MODEL

We consider the Hamiltonian [Eq. (1) in the main text]

$$\hat{H} = \begin{pmatrix} \Delta - \frac{\hbar^2\mathbf{q}^2}{2M} & \gamma(\mathbf{q}) \\ \gamma^*(\mathbf{q}) & -\Delta + \frac{\hbar^2\mathbf{q}^2}{2M} \end{pmatrix} \tag{S1}$$

with the coupling term

$$\gamma(\mathbf{q}) = \gamma_0 - \frac{\hbar^2 q_x^2}{2m_x} - \frac{\hbar^2 q_y^2}{2m_y} + i\hbar v_z q_z. \tag{S2}$$

As mentioned in the main text, the coupling leads to the opening of a gap along the nodal loop in the $q_x - q_y$ plane at $q_z = 0$ determined by $\Delta = \hbar^2\mathbf{q}^2/2M$, apart from possible crossing points at $\mathbf{q}^w$ that satisfy the additional condition for an ellipse $\gamma_0 = \hbar^2 q_x^2/2m_x + \hbar^2 q_y^2/2m_y$. The particular form of the Hamiltonian seems natural in the case of wave vectors in the vicinity of a time-reversal invariant momentum at $\mathbf{q} = 0$. However, if the origin is centered at an arbitrary point in reciprocal space, there might also be linear terms both on the diagonal and in the off-diagonal elements. These will simply shift the location of the ellipsis and the circle (cf. Fig. 1a in the main text). In the same way, the coupling constant $\gamma_0$ can be, in principle, a complex quantity, but we consider it to be a real positive parameter here to simplify the discussions. A possible imaginary part would only shift the plane, which contains the nodal line, in the $z$-direction by $q_z^0 = -\mathrm{Im}(\gamma_0)/\hbar v_z$ and can thus be omitted by a simple redefinition of the origin of the wave vector in the $z$-direction. However, the real part of $\gamma_0$ must have the same sign as the masses $m_x$ and $m_y$, which we choose to be positive henceforth, in order to fulfill the ellipse equation. Similarly, we consider also $\Delta$ and $M$ to be positive. One notices that one has four Weyl nodes at $\mathbf{q}^w = (\pm q_x^w, \pm q_y^w, 0)$, in the form of crossing points between the circle and the ellipse, if one of the following two conditions:

$$m_x > M\frac{\Delta}{\gamma_0} > m_y \quad \text{or} \quad m_x < M\frac{\Delta}{\gamma_0} < m_y, \tag{S3}$$

is fulfilled. One then finds that the Weyl nodes are located at the coordinates

$$\hbar q_x^w = \sqrt{\frac{2m_x}{m_x - m_y}(M\Delta - \gamma_0 m_y)} \tag{S4}$$

$$\text{and} \quad \hbar q_y^w = \sqrt{\frac{2m_y}{m_y - m_x}(M\Delta - \gamma_0 m_x)} \tag{S5}$$

which are indeed real quantities as long as one of the conditions (S3) is satisfied.

An expansion around the Weyl node $\mathbf{q}^w = (\xi q_x^w, \xi' q_y^w, 0)$, in terms of the signs $\xi = \pm$ and $\xi' = \pm$ that label the four different nodes, yields the low-energy Hamiltonian

$$\hat{H}^w_{\xi,\xi'} = -\hbar \begin{pmatrix} \mathbf{v}^3_{\xi\xi'} \cdot \mathbf{k}_\parallel & \mathbf{v}^1_{\xi\xi'} \cdot \mathbf{k}_\parallel - iv_z k_z \\ \mathbf{v}^1_{\xi\xi'} \cdot \mathbf{k}_\parallel + iv_z k_z & -\mathbf{v}^3_{\xi\xi'} \cdot \mathbf{k}_\parallel \end{pmatrix}, \tag{S6}$$

where $\mathbf{k} = (\mathbf{k}_\parallel, k_z)$ is the deviation of the wave vector from the Weyl node, $\mathbf{q} = \mathbf{q}^w + \mathbf{k}$, and where we have defined the velocity vectors as

$$\mathbf{v}^1_{\xi\xi'} = \left(\xi\frac{\hbar q_x^w}{m_x}, \xi'\frac{\hbar q_y^w}{m_y}\right)$$

$$\text{and} \quad \mathbf{v}^3_{\xi\xi'} = \left(\xi\frac{\hbar q_x^w}{M}, \xi'\frac{\hbar q_y^w}{M}\right). \tag{S7}$$

The upper indices (1 and 3) here refer to the sequence of Pauli matrices. One notices that the Hamiltonian (S6) is not in its canonical form. This is due to the fact that the isoenergy lines of the Weyl cones (for $q_z = 0$) around the

points $\mathbf{q}^w$ are anisotropic ellipses, but the main axes of these ellipses do not coincide with the $q_x$- and $q_y$-axes. In order to bring the Hamiltonian to its canonical form, one therefore needs to perform a rotation of the coordinate system in the $q_x - q_y$ plane that amounts to diagonalizing the velocity matrix

$$V_{\xi\xi'} = ({}^t\mathbf{v}^3_{\xi\xi'}, {}^t\mathbf{v}^1_{\xi\xi'}) = \hbar \begin{pmatrix} \xi \frac{q_x^w}{M} & \xi \frac{q_x^w}{m_x} \\ \xi' \frac{q_y^w}{M} & \xi' \frac{q_y^w}{m_y} \end{pmatrix} \tag{S8}$$

the columns of which consist of the velocity vectors (S7). In fact, we are not interested in the actual eigenvalues $v_+$ and $v_-$ of this matrix but only in their product, which is nothing other than its determinant or equivalently the cross product of the velocity vectors,

$$v_+v_- = \det(V_{\xi\xi'}) = \xi\xi' \frac{\hbar^2 q_x^w q_y^w}{M} \left( \frac{1}{m_y} - \frac{1}{m_x} \right). \tag{S9}$$

The reason to search for the product only is twofold. First, if the magnetic field is applied in the $z$-direction (as it is the case in our experiments), the LL quantization of a Weyl fermion is only sensitive to the product of $v_+$ and $v_-$. Indeed, the low-energy LLs of the Weyl nodes below the saddle points around 8 meV [see Fig. 2(a) in the main text] and for magnetic fields below $\sim 5$ T disperse as

$$E_{\pm,n} = \pm\hbar \sqrt{2 \frac{v_{\text{eff}}^2}{l_B^2} n}, \tag{S10}$$

where $l_B = \sqrt{\hbar/eB}$ is the magnetic length and $v_{\text{eff}}^2 = |v_+v_-|$ the square of the average Fermi velocity around the Weyl nodes in the $q_z = 0$ plane.

Second, the *topological (or monopole) charge of* a Weyl node is given by the sign of the product of the velocities in the three orthogonal directions

$$C_{\xi,\xi'} = -\text{sgn}(v_z v_+ v_-) = -\xi\xi' \text{sgn}(v_z)\text{sgn}(m_x - m_y), \tag{S11}$$

where the global minus sign in the last expression simply reflects the global sign of our Weyl Hamiltonian (S6). One notices that the topological charge of a Weyl node is determined by the product $\xi\xi'$ such that the Weyl nodes related by inversion $\mathbf{q} \to -\mathbf{q}$ around $\mathbf{q} = 0$ have the same charge, as one expects for time-reversal-invariant Weyl semimetals.

We finish the discussion of the low-energy model with the evaluation of the saddle points $\mathbf{q}^{\text{sp}}$ in the dispersion relation. Because of the mirror symmetries around $q_x = 0$ and $q_y = 0$, the saddle points connecting the Weyl nodes at $\mathbf{q}^w$ are necessarily located along the $x$- and $y$-axis. For simplicity, let us consider the conduction band, the valence band being simply related to the former by particle-hole symmetry. Let us consider first $q_x = 0$. The $y$-component of the saddle-point coordinate can then simply be obtained by searching the minimum of the equation

$$E^2 = \left( \Delta - \frac{\hbar^2 q_y^2}{2M} \right)^2 + \left( \gamma_0 - \frac{\hbar^2 q_y^2}{2m_y} \right)^2 \tag{S12}$$

and is found at

$$\hbar q_y^{\text{sp}} = \pm \sqrt{\frac{2}{1/M^2 + 1/m_y^2} \left( \frac{\Delta}{M} + \frac{\gamma_0}{m_y} \right)}. \tag{S13}$$

Similarly, one finds, for the saddle points with $q_y = 0$, the $x$-component

$$\hbar q_x^{\text{sp}} = \pm \sqrt{\frac{2}{1/M^2 + 1/m_x^2} \left( \frac{\Delta}{M} + \frac{\gamma_0}{m_x} \right)}. \tag{S14}$$

The energies associated with these saddle points are given by

$$E_y^{\text{sp}} = E(0, q_y^{\text{sp}}, 0) = \frac{|\Delta M - \gamma_0 m_y|}{\sqrt{M^2 + m_y^2}}, \tag{S15}$$

and

$$E_x^{\text{sp}} = E(q_x^{\text{sp}}, 0, 0) = \frac{|\Delta M - \gamma_0 m_x|}{\sqrt{M^2 + m_x^2}} \tag{S16}$$

respectively.

## II. ELECTRONIC BAND STRUCTURE OF TAP – DISCUSSION

The electronic band structure of TaP is under intensive discussions nowadays. In many aspects, our understanding as a community remains more qualitative rather than quantitative. Nevertheless, a consensus has been established that there exists a rather large energy distance between $W_1$ and $W_2$ points. According to theoretical (DFT [1–4]) and experimental studies (transport, ARPES and optics [5–7]), this separation reaches $\Delta E_{W_2-W_1} \approx 60 - 80$ meV. This implies that the Fermi level can be located either within $W_1$ or $W_2$ cones, but not within both at the same time. This contrasts to arsenic-based Weyl semimetals (TaAs and NbAs) in which the separation is much smaller (around 20 meV [3, 4]) and both types of cones have to be considered simultaneously.

The relatively large value of $\Delta E_{W_2-W_1}$ directly affects optical properties. With the Fermi energy around the $W_1$ nodes, the $W_2$ pockets can only give rise to free electron absorption (at low energies) and to interband excitations, above the onset of $2\Delta E_{W_2-W_1} \approx 120 - 160$ meV (due to Pauli blocking), as schematically shown in Fig. S1. Vice versa, the Fermi energy placed within $W_2$ pockets would limit the contribution from the $W_1$ pockets. Nevertheless, the closely packed quartet of the $W_1$ cones around the point of the Brillouin zone seems to be a much better realization of our simple model as compared to relatively distant pairs of $W_2$ cones. This leads us to a plausible assumption that the dominant contribution to the optical response in the energy window we investigate comes from the vicinity of $W_1$, rather than $W_2$ nodes.

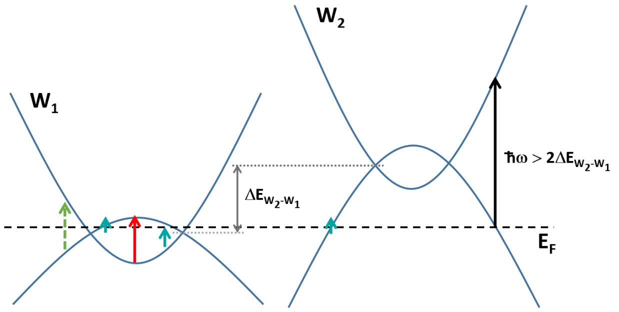


FIG. S1. Schematic view of Wey nodes in TaP. Possible optical excitations are marked by vertical arrows. The dark cyan arrows correspond to low-energy excitations, due to free carrier absorption and due to interband excitations within the $W_1$ cones. The red arrow represents excitations between minima and maxima of inverted bands. The green and black arrows correspond to interband excitations away from Weyl nodes, i.e., in the non-inverted part of the Brillouin zone. The latter excitations in the $W_2$ pocket may appear above the onset of $2\Delta E_{W_2-W_1} \approx 120 - 180$ meV.

When a magnetic field is applied, interband absorption transforms into a series of interband inter-LL excitations and free-carrier absorption into cyclotron resonance. The argument based on Pauli blocking still holds, as the Fermi energy cannot move significantly in a nearly compensated (bulk) semimetal. The two series of interband inter-LL excitations, which cross at the intermediate energy scale – well above CR modes but below the onset of $2\Delta E_{W_2-W_1}$ – must therefore originate in the same Weyl pockets. As discussed above, these pockets are most likely $W_1$.

## III. MAGNETO-TRANSPORT CHARACTERIZATION OF THE EXPLORED TAP SAMPLE

Magneto-transport measurements were performed on the sample explored optically in the main text for further characterization. As the geometry of the sample was not optimized for transport experiments, electrical contacts were simply deposited in a van der Pauw configuration on the top surface to probe approximately the optically active region.

In Fig. S2, we report the longitudinal resistance $R_{xx}$ as a function of the magnetic field applied along the [001] direction ($c$-axis) of the crystal at temperature of $T = 1.3$ K. The data were symmetrized for positive and negative magnetic fields. A positive, quadratic-like, magnetoresistance characteristic of a compensated semimetal is observed. On top of the magnetoresistance background, quantum oscillations (Shubnikov-de Haas) are observed. This can be clearly seen in the background-removed magneto-transport trace, shown in the top-left inset of Fig. S2.

Multiple frequencies contribute to the $1/B$ oscillating magnetoresistance, as confirmed by the FFT analysis (bottom-right inset of Fig. S2). This is consistent with the multiband nature of TaP [1, 3, 6]. The dominant frequency at $F = 18$ T is accompanied by secondary peaks at 10, 37, 47, and 70 T. While the frequency observed at 18 T seems to correspond well to the previously reported $\beta$ hole cross section of the Fermi surface [6], other frequencies cannot be straightforwardly assigned to the particular pockets. The differences between our sample and the ones reported by Arnold et al. [6] are actually more apparent in the angular-dependent study summarized in Fig. S3.

In the angle-dependent measurements, the sample was rotated in-situ in the magnetic field, with the angle $\theta = 0$ corresponding to the magnetic field being applied along the [001] direction (c-axis). Figure S3 shows the intensity of the individual frequency components of the FFT signal as a function of $\theta$. Around $\theta = 0$, the frequencies observed in Fig. S2 appear as warmer colors (cyan or green) in the blue background. The frequency around 10 T is only slightly smaller that the $\alpha$ neck orbit identified by Arnold et al. [6] and increases with small values of $\theta$, similar to the main (18 T) frequency. This is characteristic of an almost cylindrical Fermi surface, but both components disappear rather abruptly around $\theta = 50$ deg. The 37 T frequency also increases with $\theta$, nevertheless, no clear signal is observed at higher tilt angles, in particular in the frequency range of 50-160 T, where the $\delta$ pocket was clearly observed in Ref. 6.

Let us note that we have also performed magneto-transport measurements on a different sample coming from the same growth batch and the obtained results match those of Ref. 6 better. This suggests there exists certain variation of the Fermi surface/energy on the

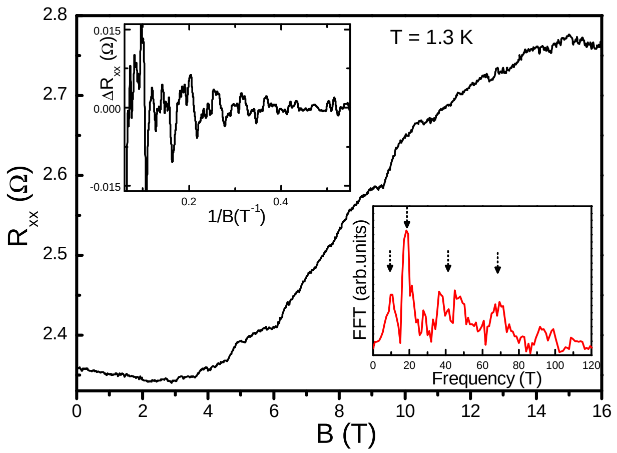


FIG. S2. Longitudinal resistance $R_{xx}$ as a function of the magnetic field at $T = 1.3$ K. Top-left inset: the removed-background signal $\Delta R_{xx}$ as a function of the inverse magnetic field. Bottom-right inset: the FFT signal with multiple spectral contributions.

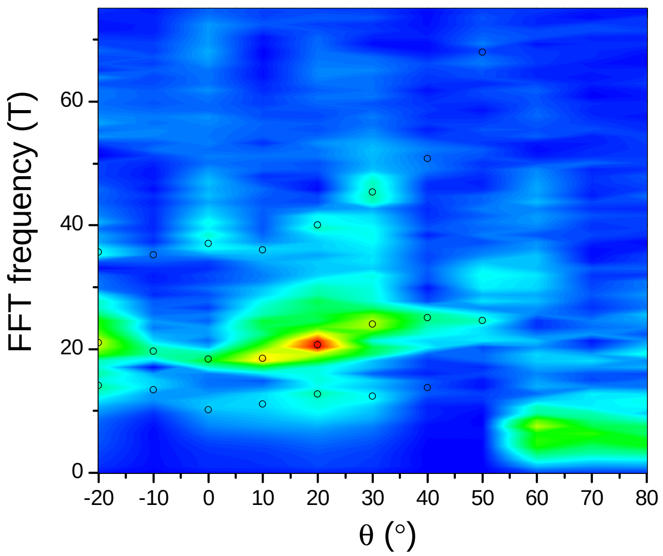


FIG. S3. Angular dependence of the FFT signal intensity. Color scale: blue to red corresponds to low to high value in arbitrary units. $\theta$ is the angle between the magnetic field and the [001] crystallographic direction ($c$-axis). Open circles materializes the maximum FFT signal position of the main spectral components.

macroscopic scale of the crystal, most likely due to intrinsic and/or extrinsic doping. This was actually already observed in previous studies [8] where non-stoichiometry and the presence of various defects were shown to lead to significant changes of the Fermi level, and correspondingly, of measured frequencies in the quantum-oscillations experiments.

As a matter of fact, the great sensitivity of the Fermi surface parameters, with respect to the Fermi level position, is a direct consequence of the rapidly varying band structure around the $W_1$ and $W_2$ Weyl points in TaP. For the studied sample, the measured Fermi surface parameters (and in particular the strong oscillating behavior at $F = 18$ T) are consistent with the Fermi level lying between the 2 Weyl points $W_1$ and $W_2$, but more precise positioning cannot be extracted from the present sample.

[1] H. Weng, C. Fang, Z. Fang, B. A. Bernevig, and X. Dai, Weyl semimetal phase in noncentrosymmetric transition-metal monophosphides, Phys. Rev. X **5**, 011029 (2015).

[2] C.-C. Lee, S.-Y. Xu, S.-M. Huang, D. S. Sanchez, I. Belopolski, G. Chang, G. Bian, N. Alidoust, H. Zheng, M. Neupane, B. Wang, A. Bansil, M. Z. Hasan, and H. Lin, Fermi surface interconnectivity and topology in Weyl fermion semimetals TaAs, TaP, NbAs, and NbP, Phys. Rev. B **92**, 235104 (2015).

[3] D. Grassano, O. Pulci, A. M. Conte, and F. Bechstedt, Validity of Weyl fermion picture for transition metals monopnictides TaAs, TaP, NbAs, and NbP from ab initio studies, Sci. Rep. **8**, 3534 (2018).

[4] D. Grassano, O. Pulci, and F. Bechstedt, Infuence of anisotropy, tilt and pairing of Weyl nodes: The Weyl semimetals TaAs, TaP, NbAs, and NbP, arXiv:1906.12231 (2019).

[5] N. Xu, H. Weng, B. Lv, C. E. Matt, J. Park, F. Bisti, V. N. Strocov, D. Gawryluk, E. Pomjakushina, K. Conder, *et al.*, Observation of weyl nodes and fermi arcs in tantalum phosphide, Nature Comm. **7**, 11006 (2016).

[6] F. Arnold, C. Shekhar, S.-C. Wu, Y. Sun, R. D. Dos Reis, N. Kumar, M. Naumann, M. O. Ajeesh, M. Schmidt, A. G. Grushin, *et al.*, Negative magnetoresistance without well-defined chirality in the Weyl semimetal TaP, Nature Commun. **7**, 11615 (2016).

[7] S.-I. Kimura, H. Yokoyama, H. Watanabe, J. Sichelschmidt, V. Süß, M. Schmidt, and C. Felser, Optical signature of Weyl electronic structures in tantalum pnictides Ta$pn$ ($pn$ = P, As), Phys. Rev. B **96**, 075119 (2017).

[8] T. Besara, D. A. Rhodes, K.-W. Chen, S. Das, Q. R. Zhang, J. Sun, B. Zeng, Y. Xin, L. Balicas, R. E. Baumbach, E. Manousakis, D. J. Singh, and T. Siegrist, Coexistence of Weyl physics and planar defects in the semimetals TaP and TaAs, Phys. Rev. B **93**, 245152 (2016).
